# Supplementary material for: Loss Landscape Dependent Self-Adjusting Learning Rates in Decentralized Stochastic Gradient Descent
Source: arXiv:2112.01433 source file (2021-12-02)
Supplement: Supplementary file 1 [file appendix-mingrui.tex]

\section{Appendix: Noise in DPSGD helps escape saddle points}
\label{appendix:saddle}
In this section, we consider a simple synthetic problem to illustrate the effect of escaping saddle points of DPSGD. The optimization problem we consider is $\min_{x_1,x_2}\mathbb{E}_{\xi}\left[(x_1^2-x_2^2)\xi\right]$, where $-1\leq x_1\leq 1,-1\leq x_2\leq 1$ and $\xi$ follows Gaussian distribution with mean $1$ and variance $10$. We know that $(0,0)$ is the saddle point, and $(0,1), (0,-1)$ are global optima. Stochastic gradient with batch size $B$ can be of form $\frac{1}{B}\sum_{i=1}^{B}(2x_1\xi_i,-2x_2\xi_i)$ where $\xi_i$, $i=1,\ldots,B$ are i.i.d. random variables following the same distribution as $\xi$. We compare the performance of SSGD and DPSGD. The initial point is set to be $(10^{-20}, 10^{-20})$, and the learning rate is set to be $\frac{1}{4}$ since the smoothness parameter of this objective function is 4. For SSGD, we consider batch size 10000 for estimating the gradient. For DPSGD~\citep{lian2017can}, we consider 5 machines setting, each machine calculating gradients using batch size 2000 and communicating with its left and right neighbor. The result is shown in Figure~\ref{fig:escapesaddle}. From the figure, we can see that DPSGD is able to escape saddle point while SSGD get stuck around the saddle point.
\begin{figure}
\centering
	\includegraphics[scale=0.3]{./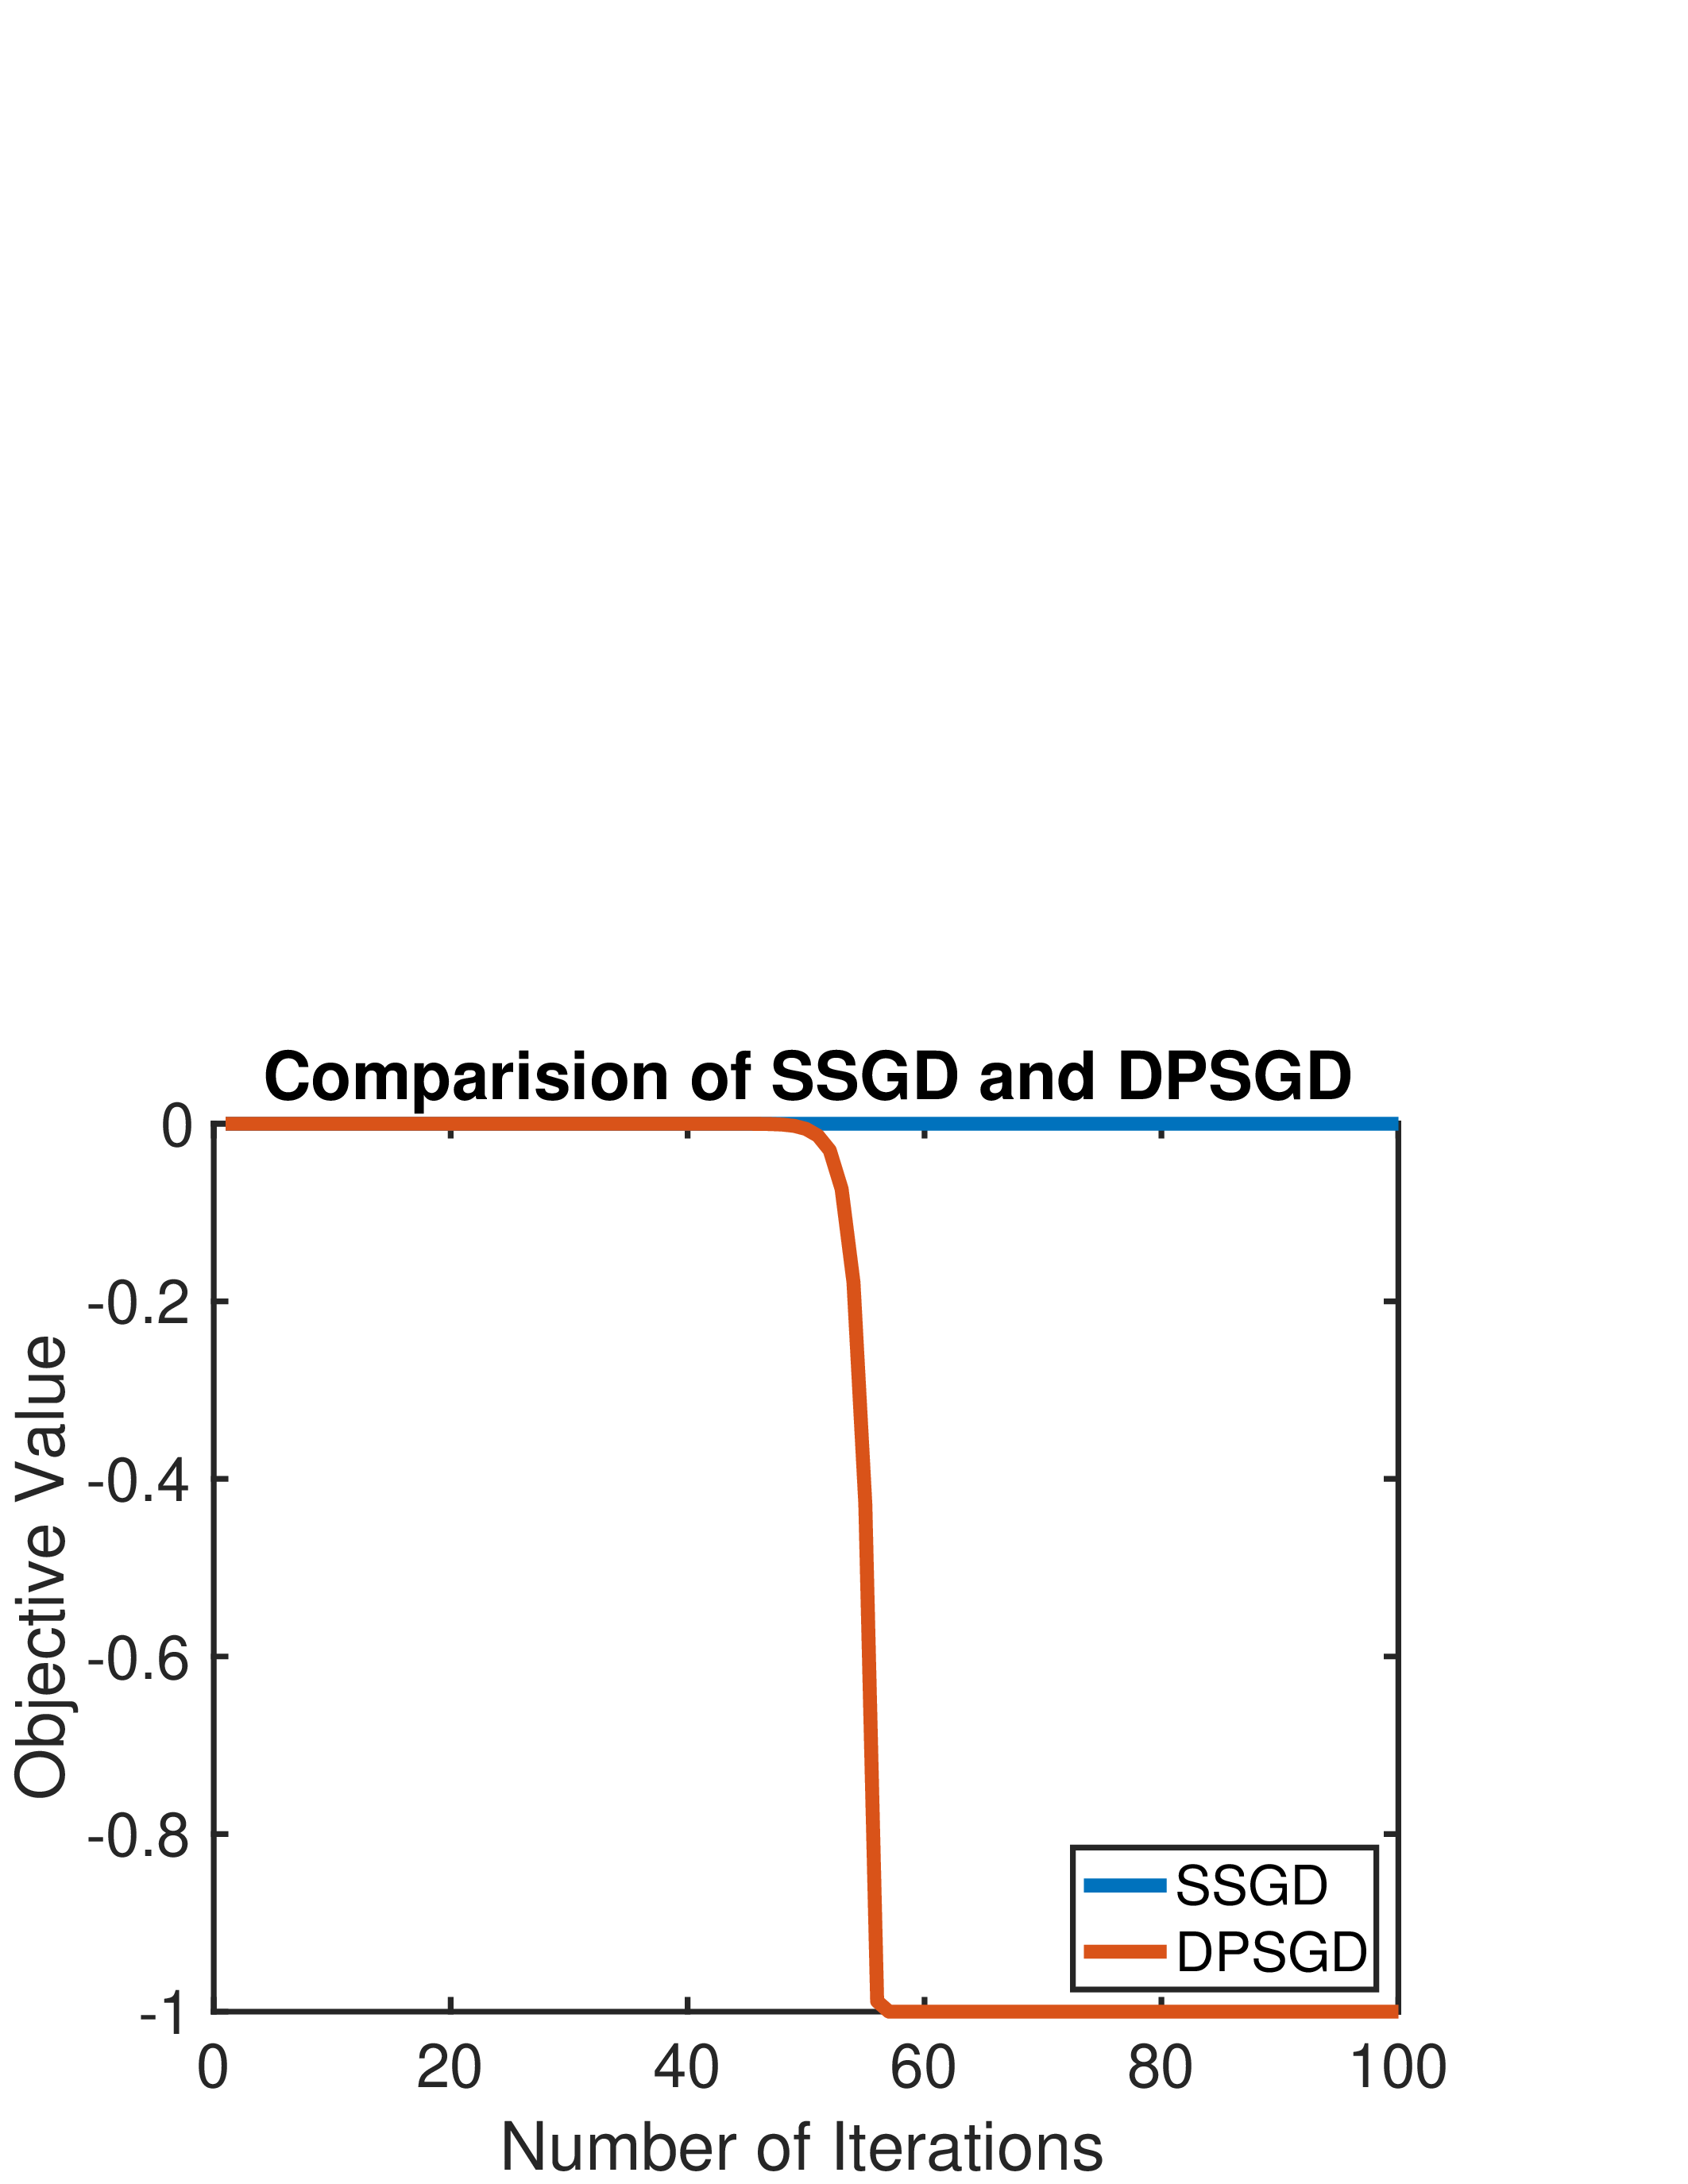}
	\caption{Comparison of SSGD and DPSGD on an synthetic example. SSGD is not able to escape saddle point $(0,0)$ while DPSGD efficiently escapes saddle point and find global optima.}
		\label{fig:escapesaddle}
\end{figure}
